# Supplementary material for: Comparative study of deep learning methods for the automatic segmentation of lung, lesion and lesion type in CT scans of COVID-19 patients
Source: arXiv:2007.15546 source file (2022-01-10)
Supplement: Supplementary file 1 [file qualitative.tex]

\subsection*{Qualitative figures for validation set}
\label{qualitative_appendix}

\begin{figure*}[htb]
    \centering
    \resizebox*{\linewidth}{!}{

    \setlength{\tabcolsep}{0pt}
    \begin{tabularx}{\linewidth}{l @{\hspace{2pt}} YYYYYYYY}

        & CT & DMLo    &  JoHof    & UNWM   & DMLu  & CTA   & WASS  & MAJ   \\

        \rotatebox{90}{\hspace{20pt} IQR25} &
        \includegraphics[width=\linewidth]{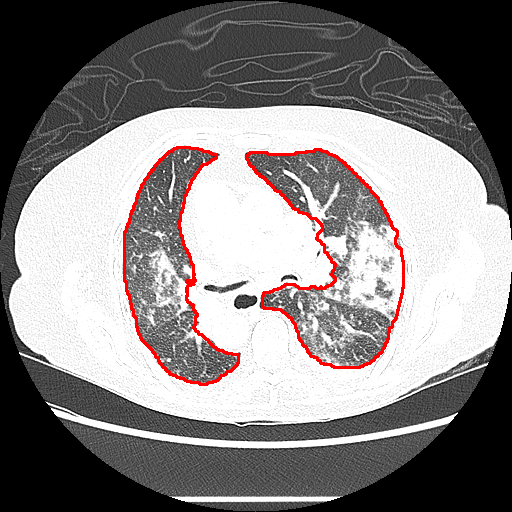} &  
        \includegraphics[width=\linewidth]{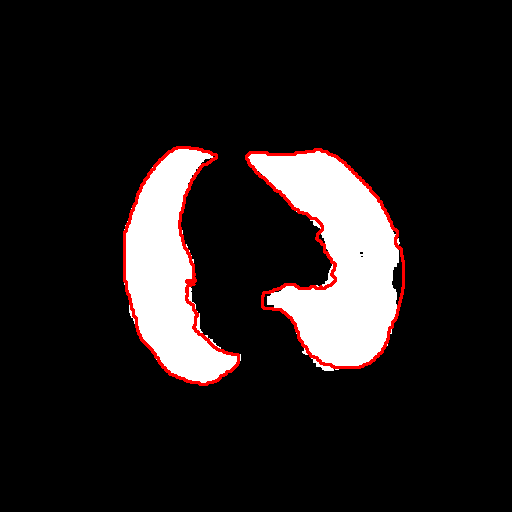} &  
        \includegraphics[width=\linewidth]{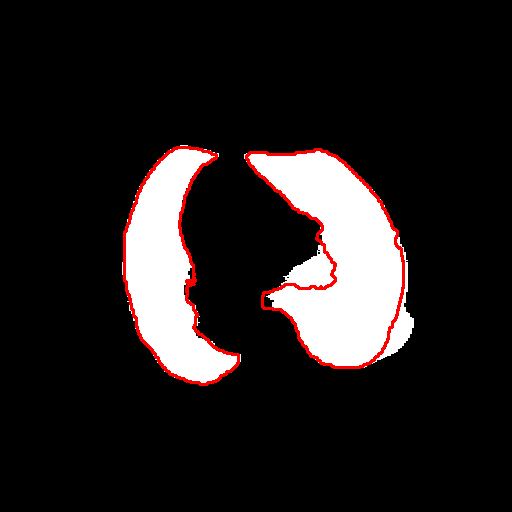} &  
        \includegraphics[width=\linewidth]{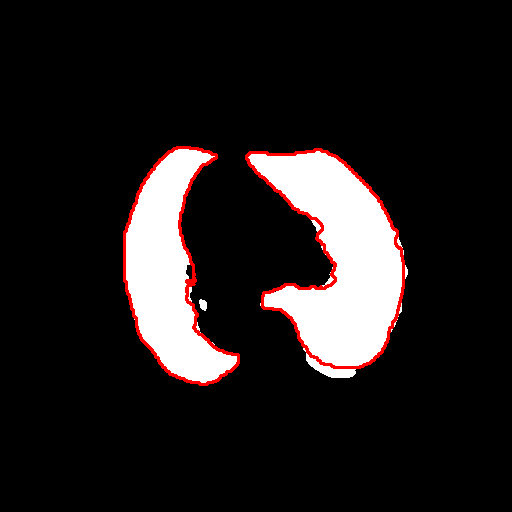} &  
        \includegraphics[width=\linewidth]{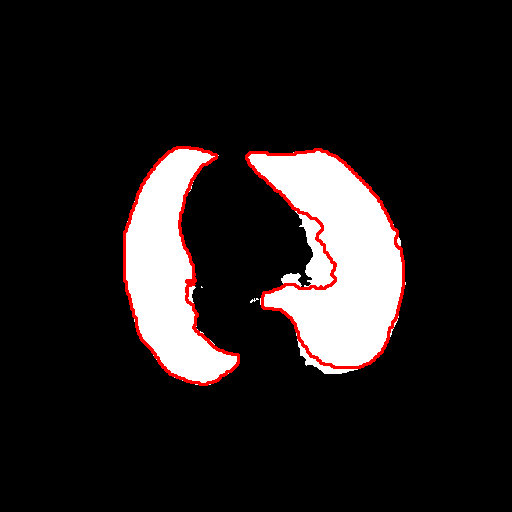} &  
        \includegraphics[width=\linewidth]{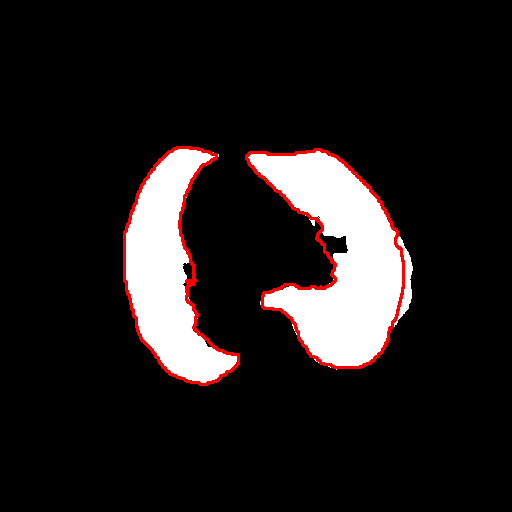} &  
        \includegraphics[width=\linewidth]{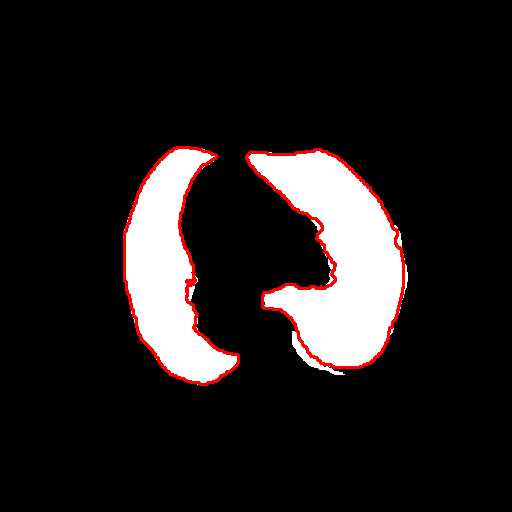} &  
        \includegraphics[width=\linewidth]{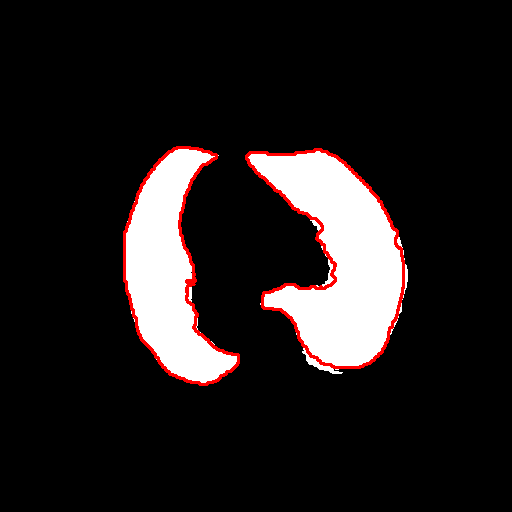} \\ 
        
        \rotatebox{90}{\hspace{20pt} MEDIAN} &
        \includegraphics[width=\linewidth]{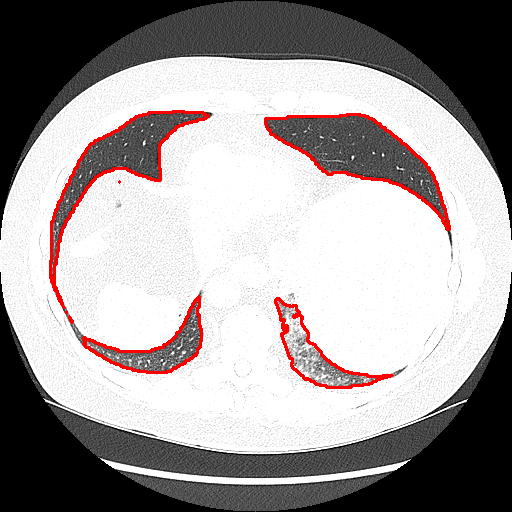} &  
        \includegraphics[width=\linewidth]{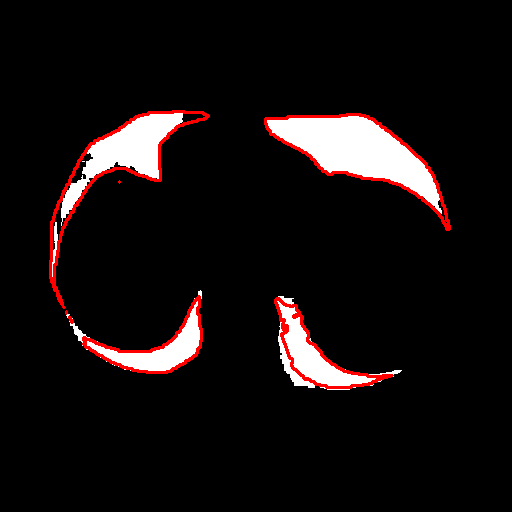} &  
        \includegraphics[width=\linewidth]{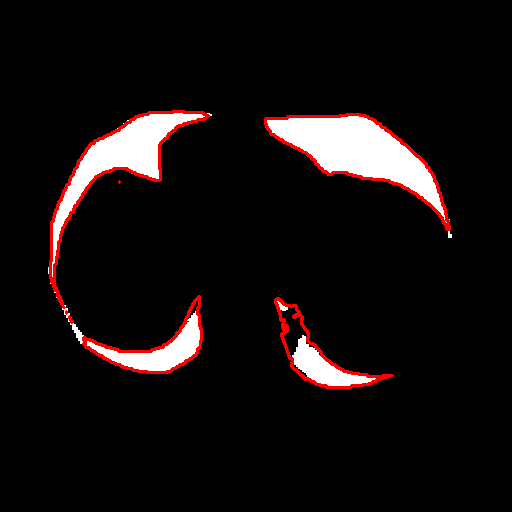} &  
        \includegraphics[width=\linewidth]{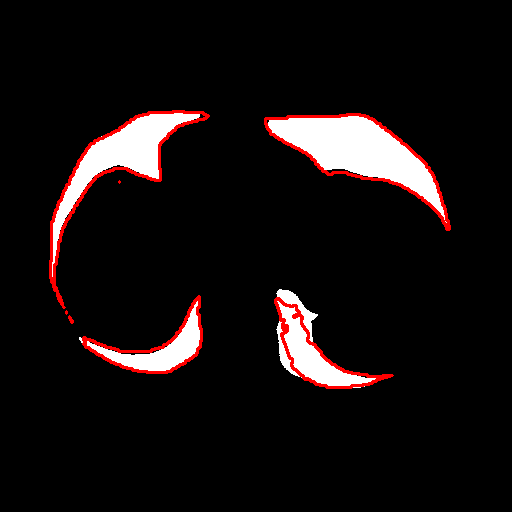} &  
        \includegraphics[width=\linewidth]{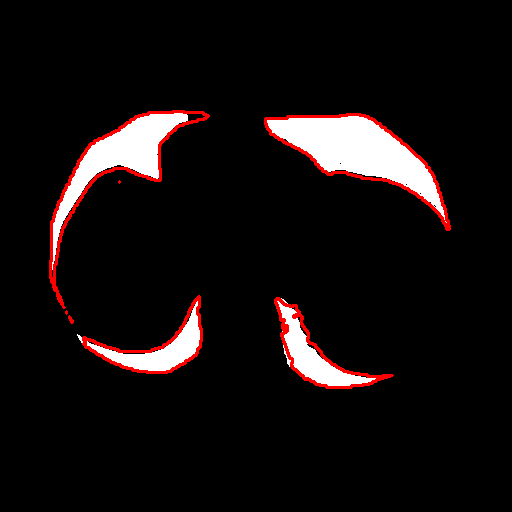} &  
        \includegraphics[width=\linewidth]{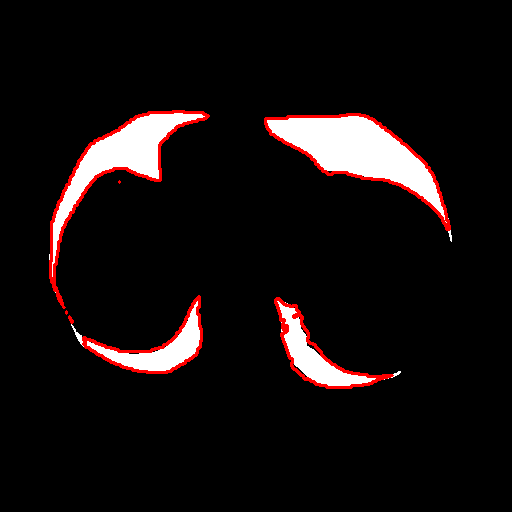} &  
        \includegraphics[width=\linewidth]{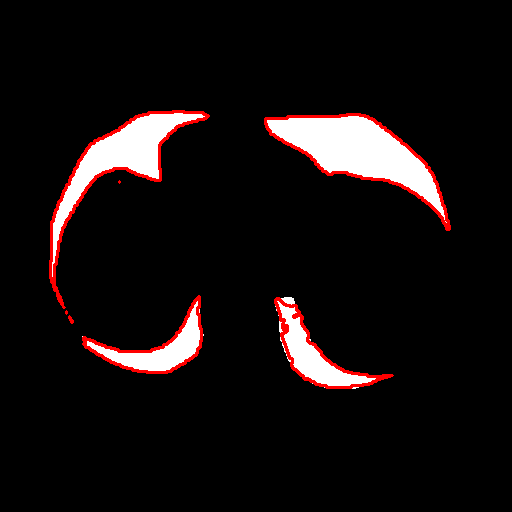} &  
        \includegraphics[width=\linewidth]{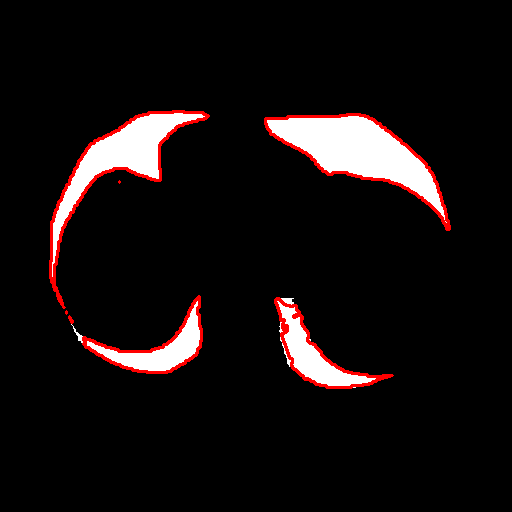} \\ 
        
        \rotatebox{90}{\hspace{20pt} IQR75} &
        \includegraphics[width=\linewidth]{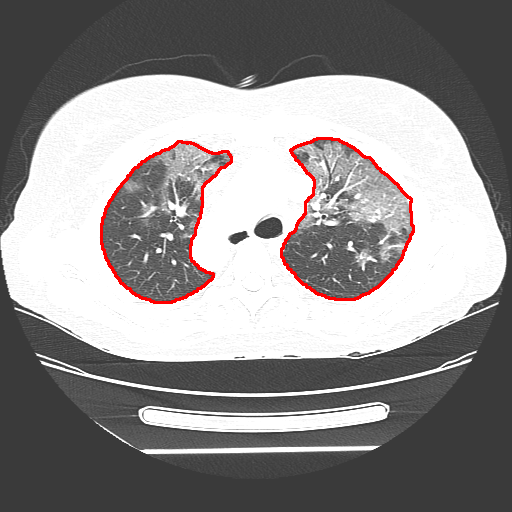} &  
        \includegraphics[width=\linewidth]{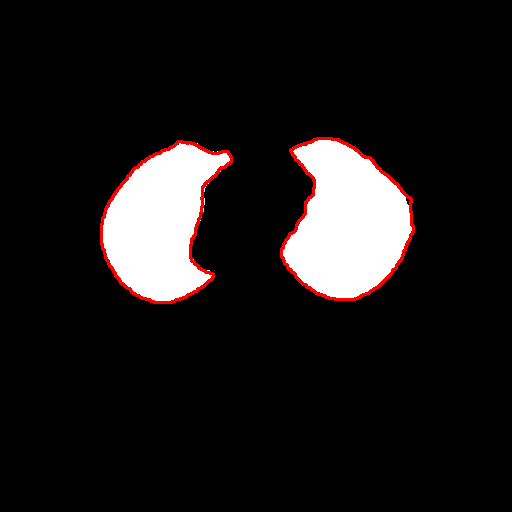} &  
        \includegraphics[width=\linewidth]{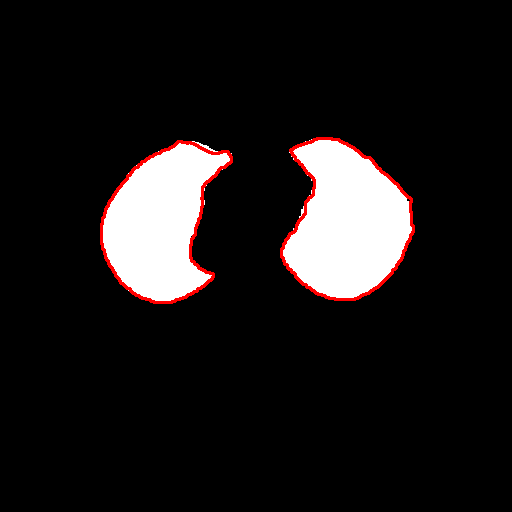} &  
        \includegraphics[width=\linewidth]{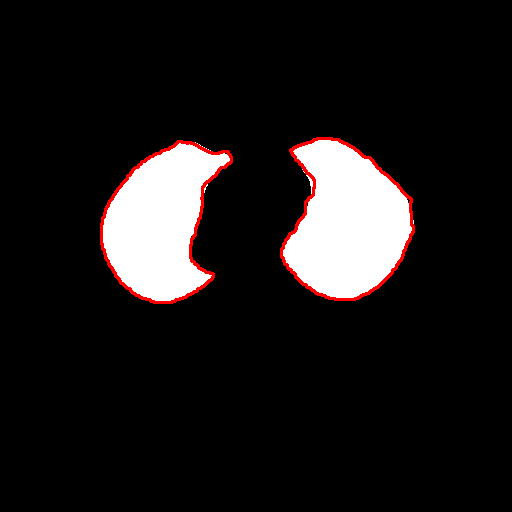} &  
        \includegraphics[width=\linewidth]{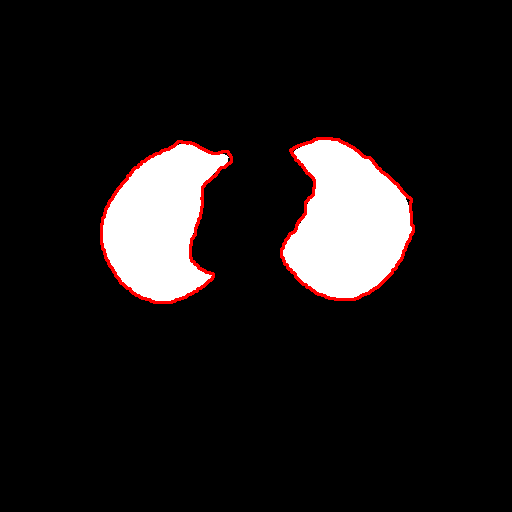} &  
        \includegraphics[width=\linewidth]{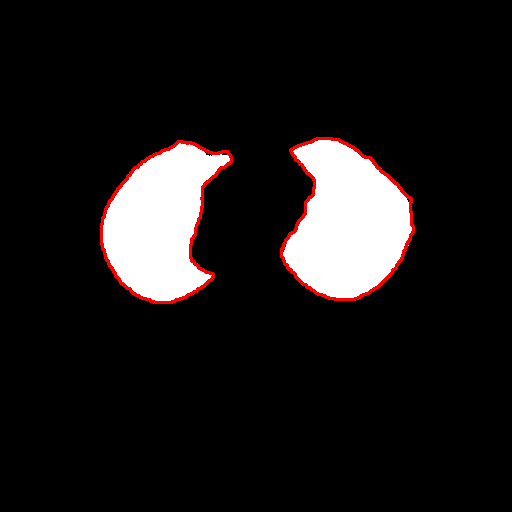} &  
        \includegraphics[width=\linewidth]{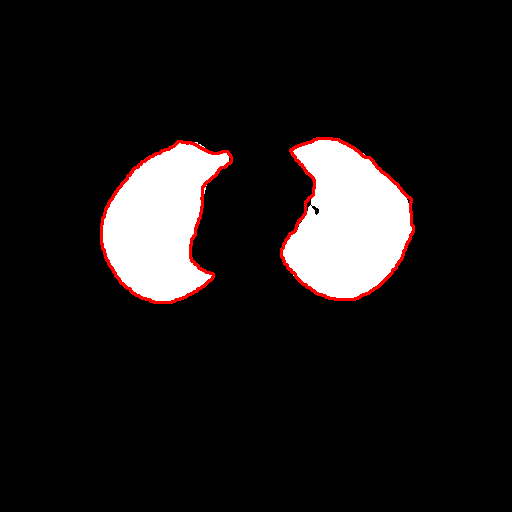} &  
        \includegraphics[width=\linewidth]{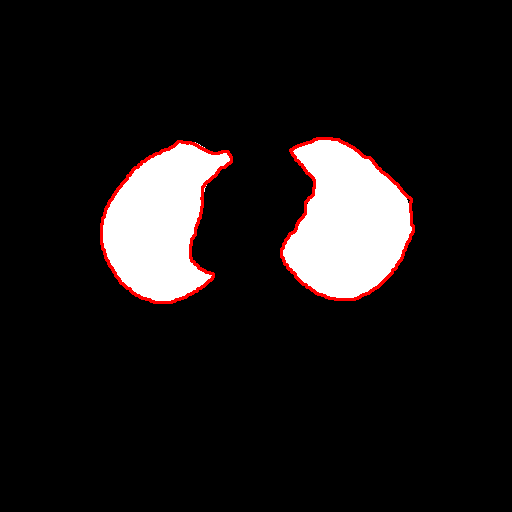} \\

    \end{tabularx}
    }
        \caption{A qualitative evaluation of the resulting predictions for lung segmentation on the validation set from each method (columns, from left to right: original CT, and predictions from DMLo, JoHof, UNWM, DMLu, CTA, WASS and MAJ). The predicted delineations are obtained after thresholding at 0.5 and each image is overlayed with the manual ground truth in red. The three rows are slices from different CT scans for which the dice score is respectively the median, first and third quartile value. The invididual slice has the median dice score among slices in that CT scan.}
    \label{fig:qualitative_master_lungs}
\end{figure*}

\begin{figure*}[htb]
    \centering
    \resizebox*{\linewidth}{!}{

    \setlength{\tabcolsep}{0pt}
    \begin{tabularx}{\linewidth}{l @{\hspace{2pt}} YYYYYYYY}

        & CT &   WASS &     2DS &     UNWM &   CTA & CENET & InfNet  &   MAJ \\
        
        \rotatebox{90}{\hspace{20pt} IQR25} &
        \includegraphics[width=\linewidth]{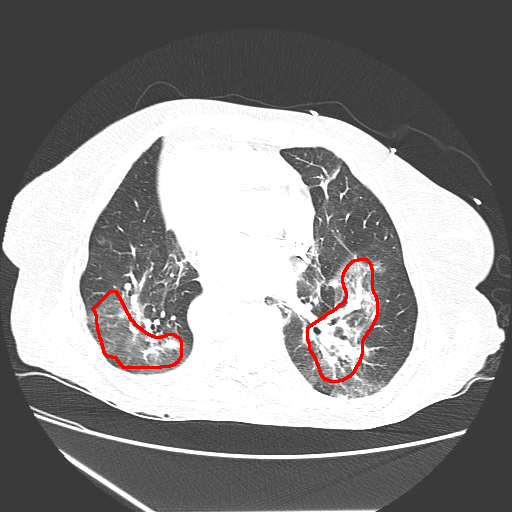} &  
        \includegraphics[width=\linewidth]{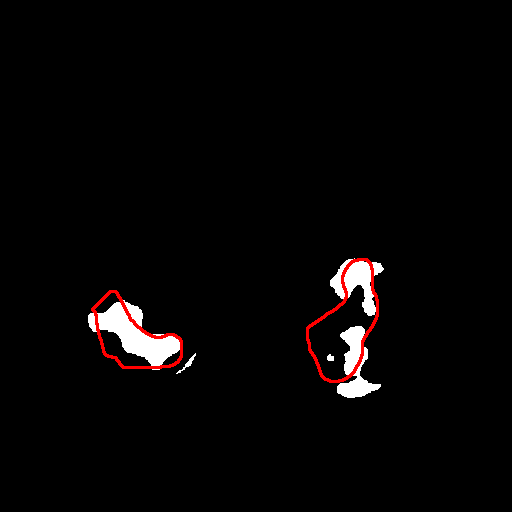} &  
        \includegraphics[width=\linewidth]{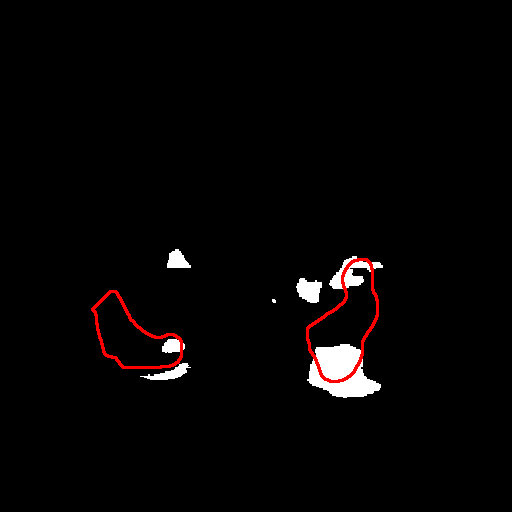} &  
        \includegraphics[width=\linewidth]{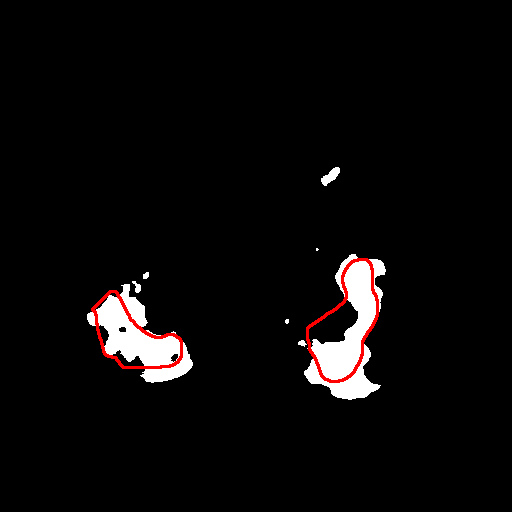} &  
        \includegraphics[width=\linewidth]{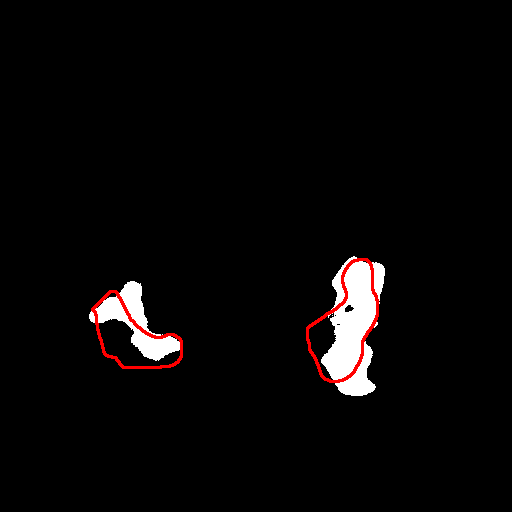} & 
        \includegraphics[width=\linewidth]{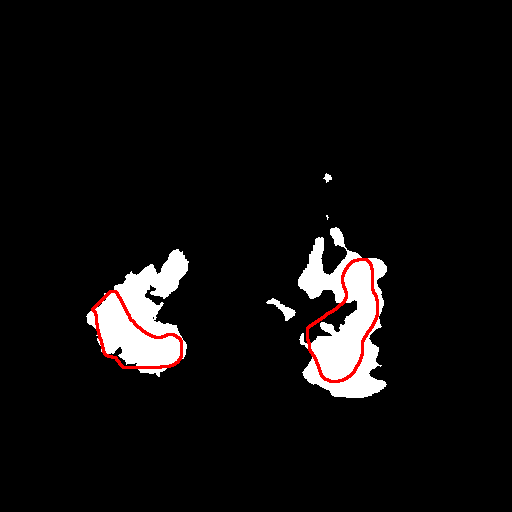} &  
        \includegraphics[width=\linewidth]{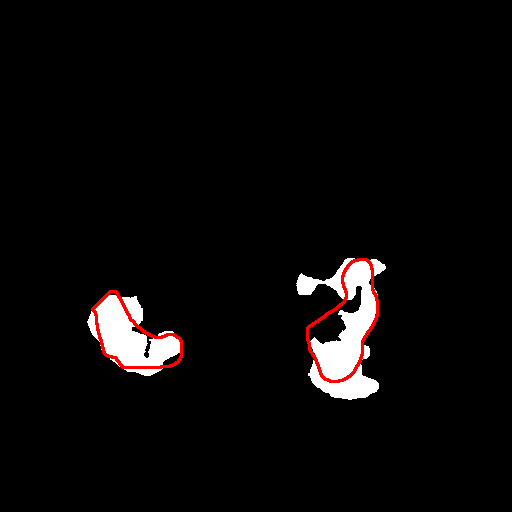} &  
        \includegraphics[width=\linewidth]{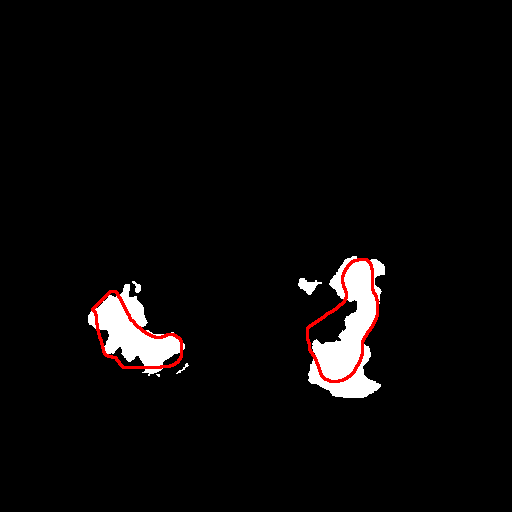} \\ 
        
        \rotatebox{90}{\hspace{20pt} MEDIAN} &
        \includegraphics[width=\linewidth]{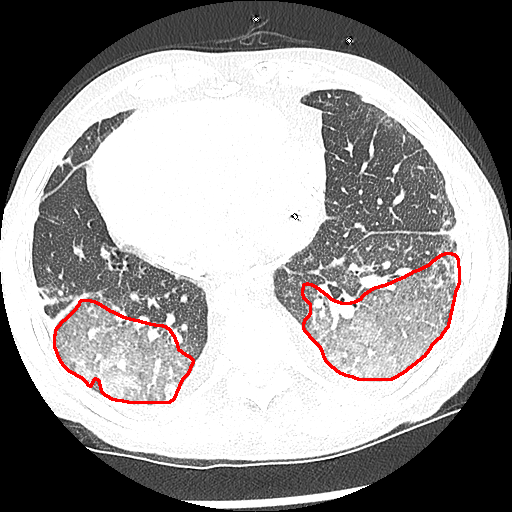} &  
        \includegraphics[width=\linewidth]{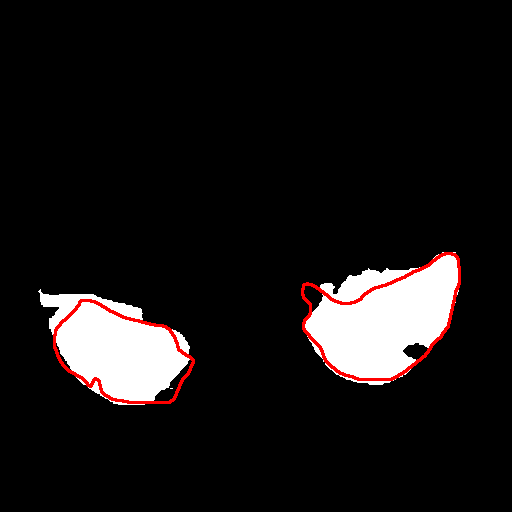} &  
        \includegraphics[width=\linewidth]{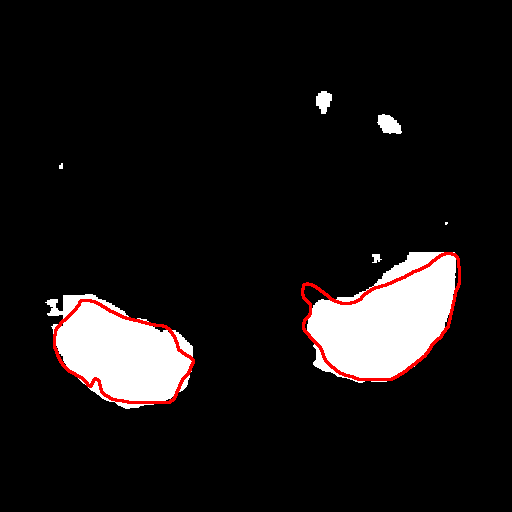} &  
        \includegraphics[width=\linewidth]{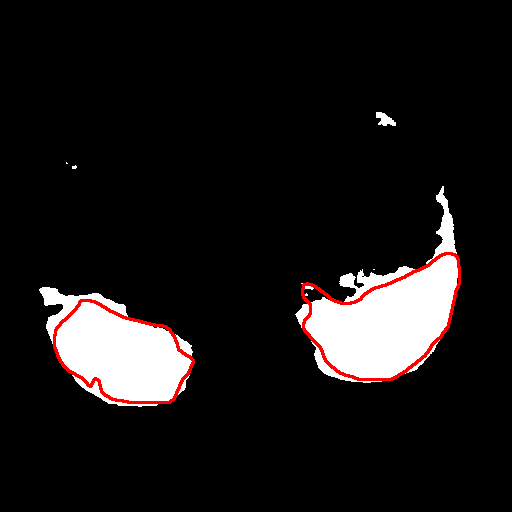} &  
        \includegraphics[width=\linewidth]{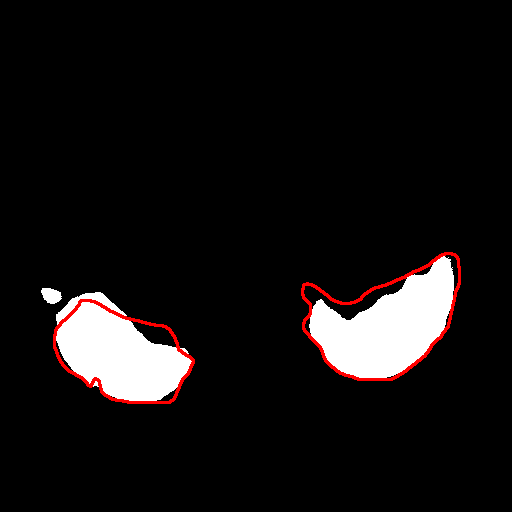} & 
        \includegraphics[width=\linewidth]{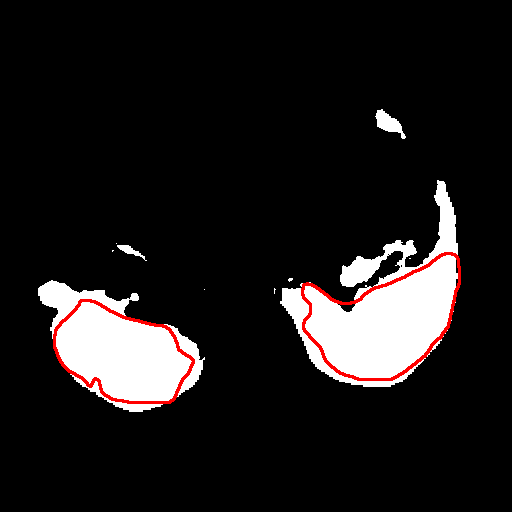} &  
        \includegraphics[width=\linewidth]{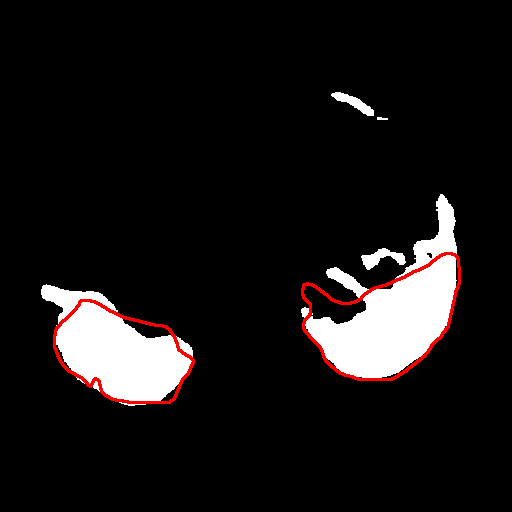} &  
        \includegraphics[width=\linewidth]{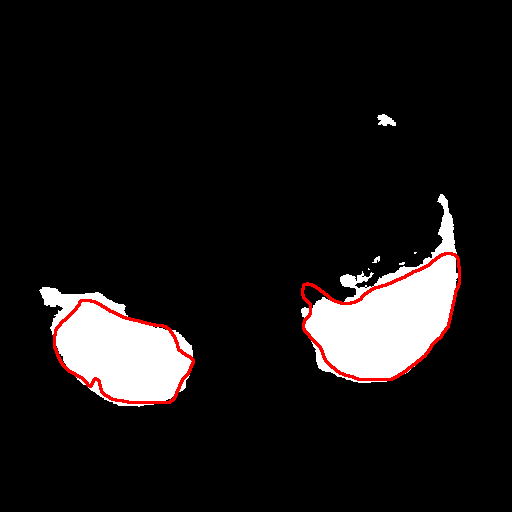} \\ 
        
        \rotatebox{90}{\hspace{20pt} IQR75} &
        \includegraphics[width=\linewidth]{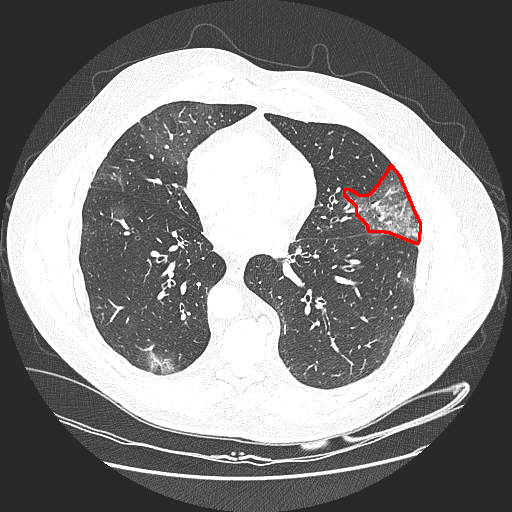} &  
        \includegraphics[width=\linewidth]{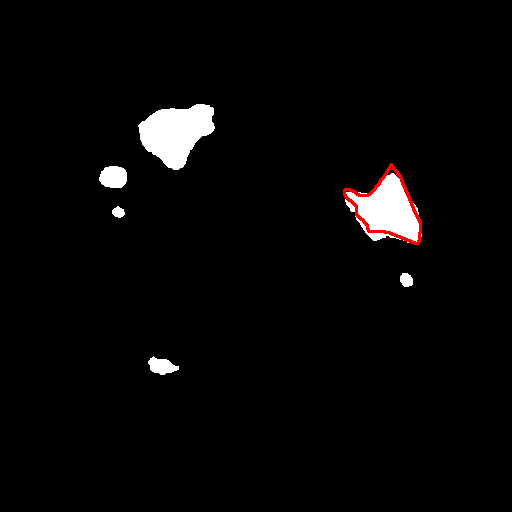} &  
        \includegraphics[width=\linewidth]{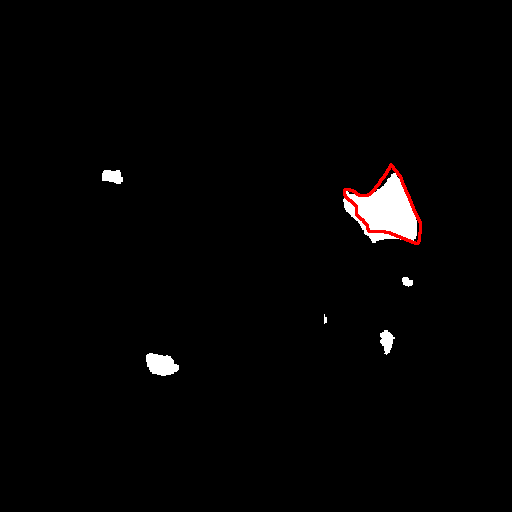} &  
        \includegraphics[width=\linewidth]{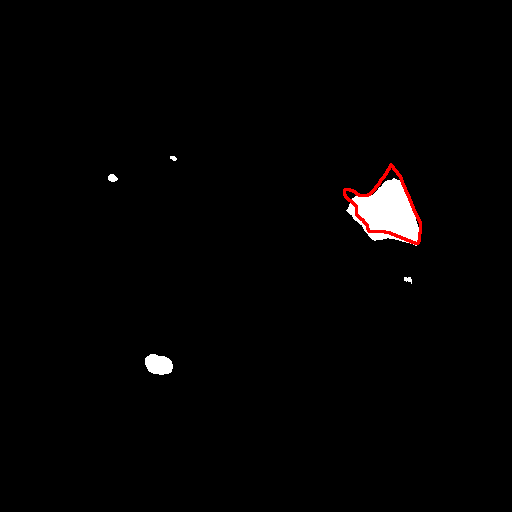} &  
        \includegraphics[width=\linewidth]{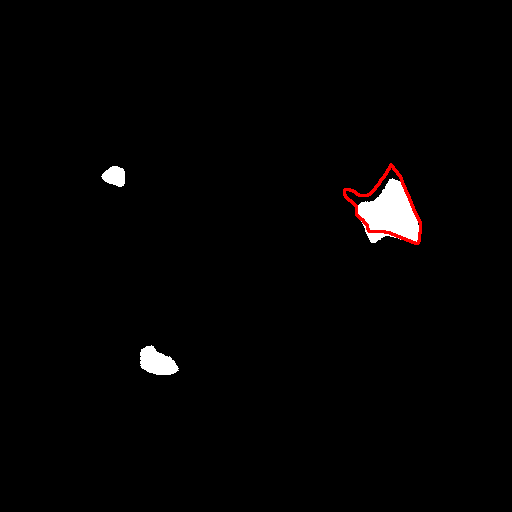} &
        \includegraphics[width=\linewidth]{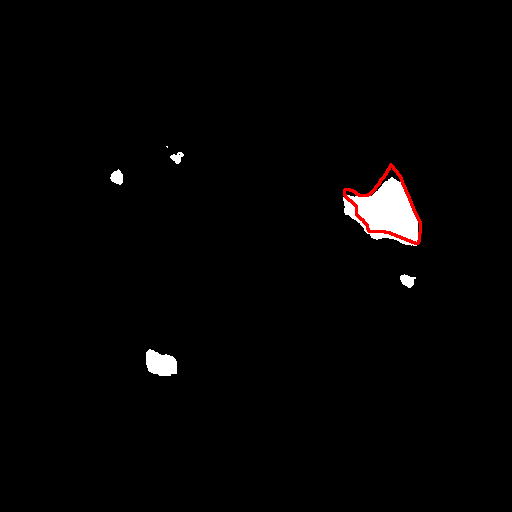} &  
        \includegraphics[width=\linewidth]{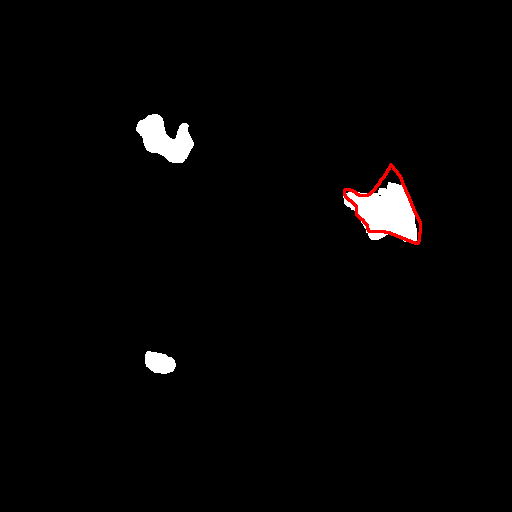} &  
        \includegraphics[width=\linewidth]{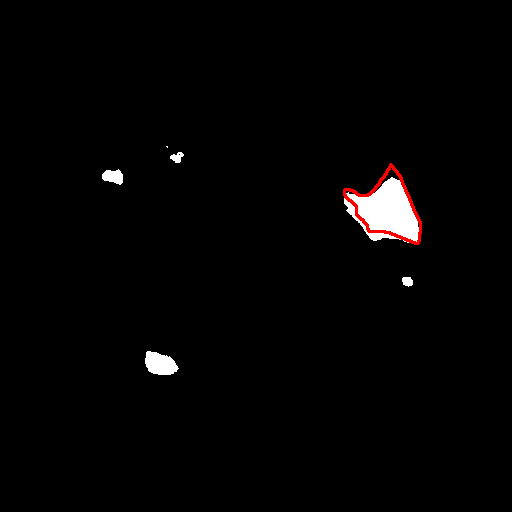} \\

    \end{tabularx}
    }
        \caption{A qualitative evaluation of the resulting predictions for lesion segmentation on the validation set from each method (columns, from left to right: original CT, and predictions from WASS, 2DS, BBB, 2Dcta and MAJ). The predicted delineations are obtained after thresholding at 0.5 and each image is overlayed with the manual ground truth in red. The three rows are slices from different CT scans for which the dice score is respectively the median, first and third quartile value. The invididual slice has the median dice score among slices in that CT scan.}
    \label{fig:qualitative_master_bin}
\end{figure*}

\input{figures/master_qualitative_mc}
